# Supplementary material for: Learning Neural Parametric Head Models
Source: arXiv:2212.02761 source file (2023-04-14)
Supplement: Supplementary file 2 [file supp_snapshot.tex]

\section{Joint Fitting}
\label{sec:joint_fitting}

- TODO Table

- TODO figure

- TODO explanation, also highlight different indications of experiments

-
